# Supplementary material for: Dynamical representations of constrained multicomponent nonlinear Schr\"odinger equations in arbitrary dimensions
Source: arXiv:2106.08010 ancillary file (2021-06-15)
Supplement: Supplementary file 1 [file DFPM_2D_NLSE.pdf]

```

% DFPM_2D_NLSE.m % Used for Figs. 4 and 5 in:
% M. Gulliksson and M. \{"O}gren, Journal of Physics A: Mathematical and Theoretical ✓
54, (2021) 275304.
% https://doi.org/10.1088/1751-8121/ac0506

% 2D 1-component nonlinear Schroedingerequation with different different constraints.

clear all; close all; clc

constant_rotation = 1 % If this is 1 the angular momentum is not constrained.
project_normalization = 1 % If this is 1 the normalization is projected to unity in ✓
each iteration.
% In Fig. 4 we used (1,1) above, while in Fig. 5 we used (0,0). The case (1,0) is not ✓
implemented.

% Physical parameters
m=1; % Mass.
hbar=1;
omega_x=1; omega_y=omega_x; % Trapping frequencies for a 2D Harmonic oscillator.
V_q = 0*0.05; % Strength of quartic part of the potential. See e.g. Phys. Rev. A 69, ✓
053619 (2004).

g = 500; % Parameter for quadratic- (GPE) nonlinearity.
eta = 4; kvec = 1*[1;1]; % Damping parameters for DFPM and for the two dynamical ✓
constraints.

% Define the vector with different \ell values to loop over.
%ell_vector = [0.2 0.8 1]; % ell_vector = [1.1 1.5 1.9];
ell_vector = [ 1]; % When constant_rotation = 1, this parameter value have no effect.
nof_ell = length(ell_vector);
Omega=0.5*ones(1,nof_ell); % Omega=[0.5 0.56 0.6] % Rotational frequency.

% Numerical tolerance and maximum number of iterations for the DFPM iteration.
tol = 1e-7; itermax = 1e5;

% Spatial Discretisation
N=129; % Number of points in x- and y-directions.
x_max=10; % Sets the size of the computational domain.
dx=(x_max-(-x_max))/(N-1); dy=dx;
x=-x_max:dx:x_max; y=x;
[X,Y]=meshgrid(x,y);

% Step size in Fictitious time.
dtau = 0.5*dx; % 1e-1; % Needs to be adjusted in relation to dx=dy.

% A function that returns the inner product of square integrable functions u and v.
dotProd2D = @(u,v,x,y,N) u'*v*dx*dy; % Use external function files instead for Octave.

% Set up matrices for the operators H_lin, L, and L^2.
V=0.5*m*(omega_x^2*X.^2 + omega_y^2*Y.^2 + V_q*(X.^2 + Y.^2).^2 ); % External ✓
potential.

H_lin=spalloc(N*N,N*N,10*N);
H_lin= 4*speye(N*N)-spdiags(ones(N*N,1),-1,H_lin)-spdiags(ones(N*N,1),1,H_lin)-...

```

```

    spdiags(ones(N*N,1),-N,H_lin)-spdiags(ones(N*N,1),N,H_lin); % 2D Laplacian.
H_lin=H_lin*hbar^2./(2*m*dx^2) + spdiags(reshape(V,[],1),0,N*N,N*N);

% Used for the L operator below.
Dx_1D = 1/dx*( -0.5*spdiags(ones(N,1),-1,N,N) + 0.5*spdiags(ones(N,1),1,N,N) ); % 1D central differences without boundary corrections.
Dx = kron(Dx_1D,speye(N)); Dy = kron(speye(N),Dx_1D); % Partial derivatives in 2D, see e.g. https://se.mathworks.com/matlabcentral/fileexchange/72241-finite-difference-matrix-for-1d-and-2d-problem
X_matrix = spdiags(reshape(X,[],1),0,N*N,N*N); Y_matrix = spdiags(reshape(Y,[],1),0,N*N,N*N);

L = ( -1i*hbar*( X_matrix*Dy - Y_matrix*Dx ) ); % Operator for L, see Eq. (78).
LL = L*L; % Operator for L^2.

phi_ho_0 = 1/sqrt(pi)*exp(-X.^2/2).*exp(-Y.^2/2); % Used to set the initial conditions below.
phi_ho_v = 1/sqrt(pi)*(X + 1i*Y).*exp(-X.^2/2).*exp(-Y.^2/2);

tic; % Start to clock the computational time for the iterations.
% Loop over different ell_0 (or Omega) values.
for ell_index = 1:nof_ell
    ell_0 = ell_vector(ell_index) % Present ell_0 value.

    % Initial wavefunction and initial v=du/dtau. It can be changed to keep the last u, v as initial conditions if ell_index > 1.
    phi_rot_Bao = (1-Omega(ell_index))*phi_ho_0 + Omega(ell_index)*phi_ho_v;
    u = reshape( phi_rot_Bao ,[],1);
    u=u/sqrt( dotProd2D(u,u,x,y,N)); % Normalize the initial condition, see Eq. (81).
    v=zeros(N*N,1); % Initial condition for v=du/dtau.

    % Iteration counter for iterative solution.
    convcond = Inf; iter = 1;
    while convcond > tol && iter < itermax
        u_old=u; % To be used for a norm below.
        if project_normalization == 1
            u=u/sqrt( dotProd2D(u,u,x,y,N)); % Normalize u in each iteration.
        end % if
        % Functional derivative of Eq. (75).
        Hq = H_lin*u + g*abs(u).^2.*u; % See Eq. (76).

        if constant_rotation == 1 && project_normalization == 1
            conj_u_u_u = abs(u).^2.*u; % Used two times below.
            E_sol_temp = real( dotProd2D(u, H_lin*u + g/2*conj_u_u_u ,x,y,N) );
            L_u = L*u; % Used two times below.
            ell_sol_temp = real( dotProd2D(u,L_u,x,y,N) ); %
            lambda_1_temp = E_sol_temp - Omega(ell_index)*ell_sol_temp + g/2*real( dotProd2D(u, conj_u_u_u ,x,y,N) );
            RHS = -Hq - [-u -L_u]*[lambda_1_temp; Omega(ell_index)] - eta*v;
            v_dtau = RHS;
            term_1 = real( dotProd2D(u, v_dtau + eta*v,x,y,N) );
            lambda_1_temp_2 = lambda_1_temp + term_1;
            lambda_1=[lambda_1_temp_2; Omega(ell_index)];
        end % if
    end
end

```

```

% Defining the constraint functions of Eq. (77).
G(:,1) = 1 - dotProd2D(u,u,x,y,N); % Norm for c_1=1.
G(:,2) = ell_0 - dotProd2D(u,L*u,x,y,N); % Angular momentum for c_2=ell_0.

if constant_rotation == 0 && project_normalization == 0
    % Define quantities needed for the Lagrange parameters.
    N_1 = real( 1 - G(:,1) );
    ell = real( ell_0 - G(:,2) );
    ell_two = real( dotProd2D(u,LL*u,x,y,N) ); % <u,L^2 u>.

    % Matrix A in Eq. (62), and vector b in Eq. (63).
    A = [N_1 ell ; ell ell_two];
    b_1 = real( kvec(1)*G(1)/2 + dotProd2D(u,Hq,x,y,N) - dotProd2D(v,v,x,y,N) ); % Only the real part is relevant since the two Lagrange parameters here are real.
    L_u = L*u; % Used two times below.
    b_2 = real( kvec(2)*G(2)/2 + dotProd2D(Hq, L_u,x,y,N) - dotProd2D(v, L*v, x,y,N) );

    % Solve for the two Lagrange parameters.
    % lambda = A\b_1; % Numerically.
    lambda = ( 1/(N_1*ell_two-ell^2)*[ b_1*ell_two - b_2*ell ; b_2*N_1 - b_1*ell ] ); % Analytic formula (Cramer's rule), faster.
    RHS = -Hq + [u L_u]*lambda - eta*v;
end % if

if constant_rotation == 1 && project_normalization ~= 1
    disp('This case is not implemented'); return
end % if

if constant_rotation ~= 1 && project_normalization == 1
    ell = real( ell_0 - G(:,2) );
    ell_two = real( dotProd2D(u,LL*u,x,y,N) ); % <u,L^2 u>
    dEduu = real( dotProd2D(Hq,u,x,y,N) ); % <dEdu,u>
    L_u = L*u; % Used two times below.
    dEduLu = real( dotProd2D(Hq,L_u,x,y,N) ); % <dEdu,Lu>
    vLv = real( dotProd2D(v,L*v) ); % <dudt,Ldudt>

    % Calculate lambda(2) from Eq. (60)
    lambda(1) = 0; % Not active.
    lambda(2) = real( ( kvec(2)*G(2)/2 + dEduLu - ell*dEduu/1 - vLv ) / ( ell_two - ell^2/1 ) );

    % Left hand side before projection
    RHS = -Hq + lambda(2)*L_u;
    % Project according to formula (59)
    RHS = RHS - u.*dotProd2D(u,RHS,x,y,N)/1 - eta*v;
end % if constant_rotation ~= 1 && project_normalization == 1

% Symplectic Euler, see Eq. (68).
v = v + dtau*RHS;
u = u + dtau*v;

% Calculate the distance from a solution:
convcond = real( sqrt( dotProd2D(RHS,RHS,x,y,N) ) );
DFPM_convergence_matrix(iter, ell_index) = convcond;

```

```

    % Save L^2 norm for convergence of the solutions
    solution_norm_convergence_matrix(iter, ell_index) = real( sqrt( dotProd2D(u
- u_old,u - u_old,x,y,N) ) ) ;
    % Save abs-values of the constraints.
    G_1_convergence_matrix(iter, ell_index) = abs(G(:,1));
    G_2_convergence_matrix(iter, ell_index) = abs(G(:,2));

    % Update the counter.
    iter = iter + 1;
end % while

% Save converged wavefunctions and observables.
u_sol(:, ell_index) = u;
E_sol(ell_index) = real( dotProd2D(u, H_lin*u + g/2*abs(u).^2.*u ,x,y,N) ); %
Total energy according to Eq. (75).
ell_sol(ell_index) = real( dotProd2D(u,L*u,x,y,N) ); % Angular momentum according
to Eqs. (77), (78).
chmPot_sol(ell_index) = lambda(1); angVel_sol(ell_index) = lambda(2); % Lagrange
parameters.
E_rot(ell_index) = E_sol(ell_index) - Omega(ell_index)*ell_sol(ell_index); %
Energy in the rotating frame, according to Eq. (80).

% Plot figures.
fs = 20; lw = 2*2; ms = 10; % Fontsize, linewidth, and markersize, for the plots.
figure(10) % A new figure for each ell_index.
P(:,1)=abs( u_sol(:,ell_index) ).^2;
subplot(3,3,ell_index); % subplot(3,1,1);
rho = reshape(P(:,1),N,N);
imagesc(x,y,rho); % Density.
set(gca,'YDir','normal')
max(P(:,1))
min(P(:,1))
axis square
xlabel('x_1','fontsize',0.6*fs)
ylabel('x_2','fontsize',0.6*fs)
set(gca,'fontsize',0.6*fs)

if ell_index==1
    colorbar('Ticks',[1e-5 0.01 0.02 ],'TickLabels',
{'0','0.01','0.02'},,'fontsize',0.6*fs)
end

s = ['$','\ell= ', num2str(ell_sol(ell_index)), '$'];
title(s,'Interpreter','Latex','fontsize',0.8*fs)

subplot(3,3,3+ell_index); % subplot(3,1,2);
PH(:,1)=angle( u_sol(:,ell_index) );
phase_of_u = reshape(PH(:,1),N,N);
imagesc(x,y,phase_of_u); % Phase.
set(gca,'YDir','normal')
axis square
xlabel('x_1','fontsize',0.6*fs)
ylabel('x_2','fontsize',0.6*fs)
set(gca,'fontsize',0.6*fs)

```

```

    if ell_index==1
        colorbar('Ticks',[-0.999*pi 0 0.999*pi], 'TickLabels',{'-\pi', '0', '\pi'}, 'fontsize',0.6*fs)
    end

    figure % A new figure for the density and phase.
    P(:,1)=abs( u_sol(:,ell_index) ).^2;
    subplot(1,2,1);
    rho = reshape(P(:,1),N,N) ;
    imagesc(x,y,rho); % Density.
    set(gca, 'YDir', 'normal')
    max(P(:,1))
    min(P(:,1))
    axis square
    xlabel('x_1', 'fontsize',0.6*fs)
    ylabel('x_2', 'fontsize',0.6*fs)
    set(gca, 'fontsize',0.6*fs, 'Xtick',[-10 -5 0 5 10], 'Ytick',[-10 -5 0 5 10])
    colorbar('Ticks',[1e-5 0.01 0.02 ], 'TickLabels',{'0', '0.01', '0.02'}, 'fontsize',0.6*fs)

    subplot(1,2,2);
    PH(:,1)=angle( u_sol(:,ell_index) );
    phase_of_u = reshape(PH(:,1),N,N);
    imagesc(x,y,phase_of_u); % Phase.
    set(gca, 'YDir', 'normal')
    axis square
    xlabel('x_1', 'fontsize',0.6*fs)
    ylabel('x_2', 'fontsize',0.6*fs)
    set(gca, 'fontsize',0.6*fs, 'Xtick',[-10 -5 0 5 10], 'Ytick',[-10 -5 0 5 10])
    colorbar('Ticks',[-0.999*pi 0 0.999*pi], 'TickLabels',{'-\pi', '0', '\pi'}, 'fontsize',0.6*fs)

    figure(10);
    subplot(3,3,6+ell_index);
    semilogy(solution_norm_convergence_matrix(:, ell_index), 'k--', 'linewidth',0.5*lw), hold on; % Convergence.
    semilogy(G_1_convergence_matrix(:, ell_index), 'b', 'linewidth',0.5*lw), hold on; % Convergence of G_1.
    semilogy(G_2_convergence_matrix(:, ell_index), 'g-.', 'linewidth',0.5*lw), hold on; % Convergence of G_2.
    axis([0 5000 1e-6 1e0]); axis square; grid on;
    xlabel('Iterations', 'fontsize',0.6*fs); ylabel('$||\ddot{u}$', 'interpreter','latex', 'fontsize',fs);
    ylabel('Convergence', 'fontsize',fs)
    box on
    if ell_index==1
        yticks([1e-6,1e-3, 1e-0])
    else
        yticks([])
    end
    set(gca, 'fontsize',0.6*fs)

end % ell_index

toc % Report the computational time for the iterations.

```

```

figure;
for ell_index=1:nof_ell
    semilogy(DFPM_convergence_matrix(:, ell_index), 'linewidth',lw), hold on; % Convergence.
end % ell_index
grid on; xlabel('Iterations'); ylabel('$||\ddot{u}$');
||$, 'interpreter', 'latex', 'fontsize',fs); box on
title('Convergence.', 'fontsize',fs)

figure;
for ell_index=1:nof_ell
    semilogy(solution_norm_convergence_matrix(:, ell_index), 'linewidth',lw), hold on; % Convergence.
end % ell_index
grid on; xlabel('Iterations'); ylabel('$||u_{j}-u_{j-1}$');
||$, 'interpreter', 'latex', 'fontsize',fs); box on
title('new Convergence.', 'fontsize',fs)

figure;
for ell_index=1:nof_ell
    subplot(2,1,1); semilogy(G_1_convergence_matrix(:, ell_index), 'linewidth',lw), hold on; % Convergence of G_1.
    subplot(2,1,2); semilogy(G_2_convergence_matrix(:, ell_index), 'linewidth',lw), hold on; % Convergence of G_2.
end % ell_index
grid on; xlabel('Iterations'); ylabel('$|G_2|$');
$|G_2|$, 'interpreter', 'latex', 'fontsize',fs); box on
subplot(2,1,1); ylabel('$|G_1|$');
$|G_1|$, 'interpreter', 'latex', 'fontsize',fs); box on
title('Convergence of constraints.', 'fontsize',fs)

figure; hold on
plot(ell_sol, E_sol, 'b.-', 'MarkerSize',ms), grid on
ylabel('$E$', 'Interpreter', 'latex', 'fontsize',fs); xlabel('$\ell$');
$\ell$, 'Interpreter', 'latex', 'fontsize',fs); box on
title('Yrast curve', 'fontsize',fs)

figure; hold on
plot(angVel_sol, E_sol, 'b.-', 'MarkerSize',ms), grid on
ylabel('$E$', 'Interpreter', 'latex', 'fontsize',fs); xlabel('$\Omega$');
$\Omega$, 'Interpreter', 'latex', 'fontsize',fs); box on

figure
subplot(2,1,1); plot(ell_sol ,chmPot_sol, 'b.-', 'MarkerSize',ms) % The chemical potential \mu is one of the Lagrange parameters.
ylabel('\mu', 'fontsize',fs); box on
title('Lagrange parameters', 'fontsize',fs)

subplot(2,1,2); plot(ell_sol ,angVel_sol, 'r.-', 'MarkerSize',ms) % The angular velocity \Omega is one of the Lagrange parameters.
xlabel('$\ell$', 'Interpreter', 'latex', 'fontsize',fs); ylabel('\Omega', 'fontsize',fs); box on

```
