# Supplementary material for: Dynamical representations of constrained multicomponent nonlinear Schr\"odinger equations in arbitrary dimensions
Source: arXiv:2106.08010 ancillary file (2021-06-15)
Supplement: Supplementary file 2 [file DFPM_n_1D_NLSE.pdf]

```

% DFPM_n_1D_NLSE.m % Used for Figs. 1, 2 and 3 in:
% M. Gulliksson and M. \{"O}gren, Journal of Physics A: Mathematical and Theoretical ✓
54, (2021) 275304.
% https://doi.org/10.1088/1751-8121/ac0506
% Note the misprint in Eq. (74) in above, where c_1 --> <\Psi_1 | \Psi_1> and c_2 --> ✓
<\Psi_2 | \Psi_2>.

% 1D n-component nonlinear Schroedingerequation with dynamical constraints, ✓
corresponding to
% \hbar=1 for a ring (periodic BC) with radius R=1.

clear all; close all; clc; tic

n = 2; % Number of components. 'Specific' examples are given for n<=4.

ell_vector = [0.0+1e-5:0.1*1e-1:1]; % Define the vector with different \ell values to ✓
loop over.

% Damping parameters for DFPM and for the n+1 constraints.
eta = 2;
kvec = 2*ones(n+1,1);

m_vector = 1/2*ones(n,1); % Mass-vector.
% m_vector = 1/2*[1; 3]; % Test example for 2-comp. with different masses. % ell_per = ✓
M_vector'*w

% Parameters for some testcases of different NLSEs.
% w is the n-vector with w(j) 'particles' in component j, with sum_j w(j) assumed to ✓
be one, needed for normalization constraints.
% gamma is the n*n-matrix with interaction parameters, see Eq. (4).
if n==1
    w=1; % Test example for 1-component, see e.g. Eur. J. Phys. 41 (2020) 065406 ✓
    (arXiv:2002.04400 [physics.comp-ph]).
    gamma = 7.5;
elseif n==2
    w=[0.8; 0.2] % Test example for 2-components, see e.g. New J. Phys. 20, 045006 ✓
    (2018) (arXiv:1710.11441 [cond-mat.quant-gas]).
    gamma = [1250 750; 750 1250]/(pi^2);
elseif n==3
    w=[0.6; 0.3; 0.1] % Test example for 3-components.
    gamma = [1250 750 750; 750 1250 750; 750 750 1250]/(pi^2);
elseif n==4
    w = [0.4; 0.3; 0.2; 0.1] % Test example for 4-components.
    gamma = 0.5*diag(1250/pi^2*ones(1,n),0);
    for j=2:n
        for k=1:j-1
            gamma(j,k) = 750/(pi^2) ;
        end % k
    end % j
    gamma = gamma + gamma';
elseif n>4
    w=0.1*1/n*[1:n-1]'; % For example.
    w(n)=1 - sum(w); % Last component.
    gamma = 0.5*diag(1250/pi^2*ones(1,n),0);
    for j=2:n

```

```

    for k=1:j-1
        gamma(j,k) = 750/(pi^2);
    end % k
end % j
gamma = gamma + gamma'
end % elseif n>4

% Numerical tolerance and maximum number of iterations for the DFPM iteration.
tol = 1e-6; itermax = 1e4;

% Spatial discretization.
nof_x = 200; dx = (2*pi)/nof_x;
x = (-pi:dx:(pi - dx))';

% Fictitious time step.
dtau = 0.95*dx

% A function that returns the inner product of square integrable functions u and v.
dotProd = @(dx, u, v) u'*v*dx; % Use external function files instead for Octave.

% Example of initial wavefunction and v=du/dtau for ell_index = 1.
% Then it can keep the last u, v as initial conditions if ell_index > 1.
u = sqrt(w'/(4*pi)).*( 1 + exp(1i*x) ); % zeros(nof_x,n);
v = zeros(nof_x,n); % Time-derivative of u.

for ell_index=1:length(ell_vector)
    ell_0 = ell_vector(ell_index); % Different \ell values to loop over.

    % While loop for iterative solution.
    iter = 0; convcond = Inf;
    while convcond > tol && iter < itermax
        iter = iter + 1; % Counter of the iteration.
        for j=1:n
            nonlinfactor = 0;
            for k=1:n
                nonlinfactor = nonlinfactor + gamma(j,k)*abs(u(:,k)).^2; % See Eq. (4).
            end % k
            Hq(:,j) = -1/(2*m_vector(j))*derivative(dx, derivative(dx, u(:,j),-1),1) +
            ...
            2*pi*nonlinfactor.*u(:,j); % See Eq. (13).
        end % j
        % Defining the constraint functionals, see Eqs. (29)-(31).
        Gangular = 0;
        for j=1:n
            Gnorm(j) = w(j) - dotProd(dx, u(:,j), u(:,j)); % w(j)=c_j, j=1,...,n.
            Gangular = Gangular - dotProd(dx, u(:,j),-1i*derivative(dx, u(:,j),0) );
        end % j
        Gangular = Gangular + ell_0; % ell_0=c_{n+1}.
        % Define quantities needed for the Lagrange multipliers.
        ell_two = 0;
        for j=1:n
            N(j) = real(dotProd(dx, u(:,j), u(:,j))); % <\Psi_j| \Psi_j>.
            ell(j) = real( dotProd(dx, u(:,j), -1i*derivative(dx, u(:,j), 0) ) ); % <\Psi_j|L \Psi_j>.
        end % j
    end
end

```

```

    ell_two = ell_two + real( dotProd(dx, u(:,j), ...
    -1*derivative(dx, derivative(dx, u(:,j), -1), 1)) ); % \sum_j <\Psi_j|L^2
\Psi_j>.
end % j

% Define the matrix A and vector b.
% A = [N ell ; ell ell_two]; % 1-component.
A = zeros(n+1,n+1); % See Eq. (62).
for j=1:n
    A(j,j) = N(j); A(j,n+1) = ell(j); A(n+1,j) = ell(j);
end % j
A(n+1,n+1) = ell_two;

b_1=zeros(n,1); % See Eq. (63).
sum_part_2=0;
for j=1:n
    b_1(j) = real( kvec(n)*Gnorm(j)/2 + dotProd(dx, u(:,j), Hq(:,j)) ...
    - dotProd(dx, v(:,j), v(:,j)) ); % Only the real part is relevant
since the Lagrange multipliers are assumed real.
    sum_part_2 = sum_part_2 - 1i*dotProd(dx, conj( derivative(dx, u(:,j),
0)), ...
    conj(Hq(:,j))) + 1i*dotProd(dx, v(:,j), derivative(dx, v(:,j), 0));
end % j
b_2 = real( kvec(n+1)*Gangular/2 + sum_part_2 ); % See Eq. (63).

% Solve for the Lagrange parameters \lambda numerically.
lambda = A\b_1; b_2];

RHS = zeros(nof_x,n); % See Eq. (61).
for j=1:n
    RHS(:,j) = -Hq(:,j) + u(:,j)*lambda(j) - 1i*derivative(dx, u(:,j),0)*lambda
(n+1) - eta*v(:,j);
end % j

% Symplectic Euler.
v = v + dtau*RHS;
u = u + dtau*v;

% Calculate the distance from a solution.
convcond = sqrt( dotProd(dx, RHS(:), RHS(:)) );
DFPM_convergence_matrix(iter,ell_index) = convcond;

% Save abs-values of the constraints.
G_1_convergence_matrix(:,iter) = abs(Gnorm);
G_2_convergence_matrix(iter) = abs(Gangular);

end % while

% Shift the densities according to the minimum for component j at theta = 0.
% minority_component_index = n;
minority_component_index = find(w==min(w),1); % Minority component.
[~, I1] = min(abs(u(:,minority_component_index)).^2); I2 = nof_x/2 + 1; shift = I2 - I1;
u = circshift(u, shift);

```

```

% Save converged wavefunctions.
u_sol(:, :, ell_index) = u;

% Total angular momentum.
ell_final = 0;
for j=1:n
    ell_final = ell_final + dotProd(dx, u_sol(:, j, ell_index), -1i*derivative(dx, u_sol(
(:, j, ell_index), 0) ));
end % j
ell_final_vector(ell_index) = real( ell_final ); % Compare with ell_vector,
ell_final_vector-ell_vector.

% Total energy.
E_kin(ell_index) = 0; E_int(ell_index) = 0;
for j=1:n
    nonlinfactor = 0;
    for k=1:n
        nonlinfactor = nonlinfactor + gamma(j,k)*abs(u_sol(:, k, ell_index)).^2;
    end % k
    E_int(ell_index) = E_int(ell_index) + dotProd(dx, u_sol(:, j, ell_index),
pi*nonlinfactor.*u_sol(:, j, ell_index));
    E_kin(ell_index) = E_kin(ell_index) + real( dotProd(dx, u_sol(:, j, ell_index), ...
-1/(2*m_vector(j))*derivative(dx, derivative(dx, u_sol(:, j, ell_index), -1),
1) ) );
end % j
E_tot_vector(ell_index) = real( E_kin(ell_index) + E_int(ell_index) );
mu_vector(ell_index, :) = real( lambda(1:end-1) ); % Saves the n different chemical
potentials (Lagrange multipliers for normalization).
Omega_vector(ell_index) = real( lambda(end) ); % Saves the angular velocity (Lagrange
multipliers for angular momentum).

end % ell_index

toc % Stop the timer.

fs = 20; lw = 2; ms = 10; % Fontsize, linewidth, and markersize, for the plots.

normalized_yrast_curve = -E_tot_vector(1) + E_tot_vector - ell_final_vector.^2;

% Plot figures.
figure(1);
subplot(2,1,1); hold on
plot(ell_final_vector, E_tot_vector, 'g.-')
box on; set(gca, 'fontsize', fs);
xlabel('$\ell_0$', 'interpreter', 'latex', 'fontsize', fs); ylabel
('Energy', 'interpreter', 'latex', 'fontsize', fs);

subplot(2,1,2); hold on
plot(ell_final_vector, Omega_vector, '.-');
ylabel('$\Omega$', 'interpreter', 'latex', 'fontsize', fs);
xlabel('$\ell_0$', 'interpreter', 'latex', 'fontsize', fs);
box on; set(gca, 'fontsize', fs);

figure
for ell_index=1:length(ell_vector)

```

```

    density_matrices_n(:,:,ell_index) = real( conj(u_sol(:,:,ell_index)).*u_sol(:,:,ell_index) ); %
    phase_matrices_n(:,:,ell_index) = angle(u_sol(:,:,ell_index));

    test_final_normalization(:,ell_index) = (sum(density_matrices_n(:,:,ell_index)) *dx)'; % w

    subplot(2,1,1); hold on
    plot(x, density_matrices_n(:,:,ell_index) ,'.-'); ylabel
('densities','interpreter','latex','fontsize',fs);
    subplot(2,1,2); hold on
    plot(x, phase_matrices_n(:,:,ell_index) ,'.-'); ylabel
('phases','interpreter','latex','fontsize',fs);
    xlabel('$x$', 'interpreter','latex','fontsize',fs)
end % ell_index

subplot(2,1,1); xlim([-pi pi]); set(gca, 'fontsize',fs, 'xtick', [-pi 0 pi], 'XTickLabel',
{'-\pi', '0', '\pi'}); box on
subplot(2,1,2); axis([-pi pi -pi pi]); set(gca, 'fontsize',fs, 'xtick', [-pi 0
pi], 'XTickLabel', {'-\pi', '0', '\pi'}, ...
    'ytick', [-pi 0 pi], 'YTickLabel', {'-\pi', '0', '\pi'}); box on

test_normalization = test_final_normalization - w; % Check the normalization
conditions, repeated length(ell_vector) times.
test_angular_momentum = ell_final_vector - ell_vector;

figure
semilogy(DFPM_convergence_matrix(1:end-1,:))
title('Convergence of gradient of Lagrangian')
xlabel('Iterations','interpreter','latex')
set(gca, 'fontsize',fs); box on

% Calculating first order derivatives. % Could be used as a separate .m file e.g. in
Octave.
function [ dq ] = derivative(h, u, BCF)
if BCF == -1 % Backward.
    dq = (circshift(u, -1) - circshift(u, 0))/(h);
elseif BCF == 0 % Central.
    dq = (circshift(u, -1) - circshift(u, 1))/(2*h);
elseif BCF == 1 % Forward.
    dq = (circshift(u, 0) - circshift(u, 1))/(h);
end

end % function

```
